# Supplementary material for: Voltage Hysteresis of Silicon Nanoparticles: Chemo-Mechanical Particle-SEI Model
Source: arXiv:2305.17533 ancillary file (2023-07-26)
Supplement: Supplementary file 1 [file supporting-information.pdf]

# Supporting Information: Voltage Hysteresis of Silicon Nanoparticles: Chemo-Mechanical Particle-SEI Model

Lukas Köbbing
*Institute of Engineering Thermodynamics, German Aerospace Center (DLR), Wilhelm-Runge-Straße 10, 89081 Ulm, Germany and Helmholtz Institute Ulm (HIU), Helmholtzstraße 11, 89081 Ulm, Germany*

Arnulf Latz and Birger Horstmann*
*Institute of Engineering Thermodynamics, German Aerospace Center (DLR), Wilhelm-Runge-Straße 10, 89081 Ulm, Germany Helmholtz Institute Ulm (HIU), Helmholtzstraße 11, 89081 Ulm, Germany and Institute of Electrochemistry, Ulm University, Albert-Einstein-Allee 47, 89081 Ulm, Germany*

## SI. THERMODYNAMIC CONSISTENT THEORY

For the general derivation of the thermodynamic theory, we follow Kolzenberg et al. [1] and additionally introduce viscous behavior. We consider the first Piola-Kirchhoff stress $\mathbf{P}$ as the sum of the stress due to elastic deformation $\mathbf{P}_{\text{el}}$ and the stress due to viscous behavior $\mathbf{P}_{\text{visc}}$

$$\mathbf{P} = \mathbf{P}_{\text{el}} + \mathbf{P}_{\text{visc}}. \tag{S1}$$

The general momentum balance with momentum $\vec{g}$ reads

$$\rho_0 \dot{\vec{g}} = \nabla_0 \cdot \mathbf{P} + \rho_0 \vec{b}, \tag{S2}$$

where $\rho_0$ is the host density in the undeformed Lagrange frame and $\vec{b}$ are body forces. The time derivative of the total energy density $e$ is described by

$$\rho_0 \dot{e} = \rho_0 \vec{v}\vec{b} + \nabla_0 \cdot \left(\mathbf{P}^{\text{T}} \vec{v}\right), \tag{S3}$$

where $\vec{v}$ is the velocity of the host material. Next, we use the product rule $\nabla_0 \cdot \left(\mathbf{P}^{\text{T}}\vec{v}\right) = \vec{v}\nabla_0 \cdot \mathbf{P} + \mathbf{P} : \nabla_0 \vec{v}$ and recognize that $\dot{\mathbf{F}} = \nabla_0 \vec{v}$. The internal energy $u$ then changes according to $\dot{u} = \dot{e} - \vec{v}\dot{\vec{g}}$ as

$$\rho_0 \dot{u} = \mathbf{P} : \dot{\mathbf{F}}. \tag{S4}$$

The second law of thermodynamics imposes a non-negative dissipation rate $\mathcal{R} \geq 0$. The generic entropy balance reads

$$\rho_0 T \dot{s} = -\nabla T \vec{N}_{\text{S},0} + \mathcal{R} \tag{S5}$$

with the entropy flux $\vec{N}_{\text{S},0}$. We rewrite Eq. (S5) with the free energy $\varphi$ using the Legendre transformation of the internal energy $\varphi = u - Ts$ as

$$\mathcal{R} = -\rho_0 \dot{\varphi} + \mathbf{P} : \dot{\mathbf{F}} + \nabla_0 T \vec{N}_{\text{S},0} \geq 0. \tag{S6}$$

We state the total time derivative of the free energy of a mobile species in an elastic material as

$$\rho_0 \dot{\varphi} = \mu_{\text{Li}} \dot{c}_{\text{Li},0} + \frac{1}{2}\mathbf{T}_{\text{rev}} : \dot{\mathbf{C}}_{\text{rev}}. \tag{S7}$$

Here, $\mathbf{T}_{\text{rev}}$ is the reversible second Piola-Kirchhoff stress tensor only due to elastic deformation. The chemical potential $\mu_{\text{Li}}$ and the reversible second Piola-Kirchhoff stress tensor are defined as

$$\mu_{\text{Li}} = \frac{\partial(\rho_0 \varphi)}{\partial c_{\text{Li},0}} \tag{S8}$$

$$\mathbf{T}_{\text{rev}} = 2\frac{\partial(\rho_0 \varphi)}{\partial \mathbf{C}_{\text{rev}}}. \tag{S9}$$

---

* birger.horstmann@dlr.de

Combining the dissipation equation Eq. (S6) with the balance of the free energy Eq. (S7) gives

$$\mathcal{R} = -\mu_{\mathrm{Li}}\dot{c}_{\mathrm{Li},0} - \frac{1}{2}\mathbf{T}_{\mathrm{rev}} : \dot{\mathbf{C}}_{\mathrm{rev}} + \mathbf{P} : \dot{\mathbf{F}} + \nabla_0 T \vec{N}_{\mathrm{S},0} \geq 0. \tag{S10}$$

The mechanical power density is composed of a reversible part due to elastic deformation, an irreversible part due to plastic flow, and a dissipation part due to viscous behavior

$$\mathbf{P} : \dot{\mathbf{F}} = \frac{1}{2}\mathbf{T}_{\mathrm{rev}} : \dot{\mathbf{C}}_{\mathrm{rev}} + \mathbf{M} : \mathbf{L}_{\mathrm{pl}} + \mathbf{P}_{\mathrm{visc}} : \dot{\mathbf{F}}, \tag{S11}$$

where $\mathbf{M} = \mathbf{C}_{\mathrm{rev}}\mathbf{T}_{\mathrm{rev}}$ is the Mandel stress and $\mathbf{L}_{\mathrm{pl}} = \dot{\mathbf{F}}_{\mathrm{pl}}\mathbf{F}_{\mathrm{pl}}^{-1}$ is the plastic velocity gradient. Finally, we obtain an expression for the dissipation rate that guarantees non-negative entropy production

$$\mathcal{R} = -\vec{N}_{\mathrm{S},0}\nabla_0\mu_{\mathrm{Li}} + \mathbf{M} : \mathbf{L}_{\mathrm{pl}} + \mathbf{P}_{\mathrm{visc}} : \dot{\mathbf{F}} \geq 0. \tag{S12}$$

Non-negativity of the first two terms in Eq. (S12) is shown in Ref. [1], and non-negativity of the last term results from our viscosity model.

## SII. ELASTOPLASTIC THIN-FILM SILICON ANODE

Many articles discuss the voltage hysteresis in thin-film silicon anodes due to plasticity of silicon [2–9]. In this setup, silicon is deposited as a film on a current collector. This current collector restricts the expansion to the normal direction of the plane. In-plane expansion is completely prohibited by the current collector as illustrated in Fig. S1. As depicted in Fig. S2(a), large stresses occur during lithiation already for small SOC due to the restricted expansion. For slow lithiation, they are almost independent of the lithiation current. After a regime of elastic deformation, the silicon film deforms plastically at a constant Piola-Kirchhoff stress. During delithiation, the silicon shrinks elastically first and then again plastically. The plastic flow inside the silicon anode leads to dissipation and an observable voltage hysteresis in silicon thin-film electrodes as shown in Fig. S2(b).

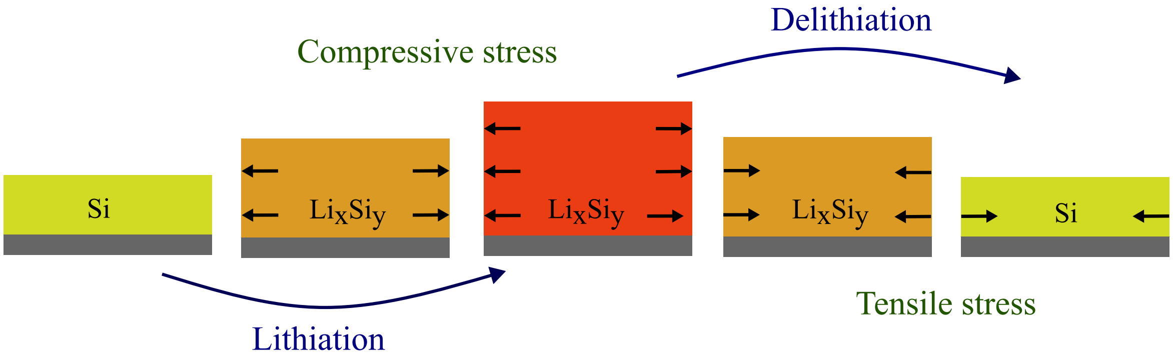


FIG. S1. Scheme of the stress inside a thin-film silicon anode during lithiation and delithiation.

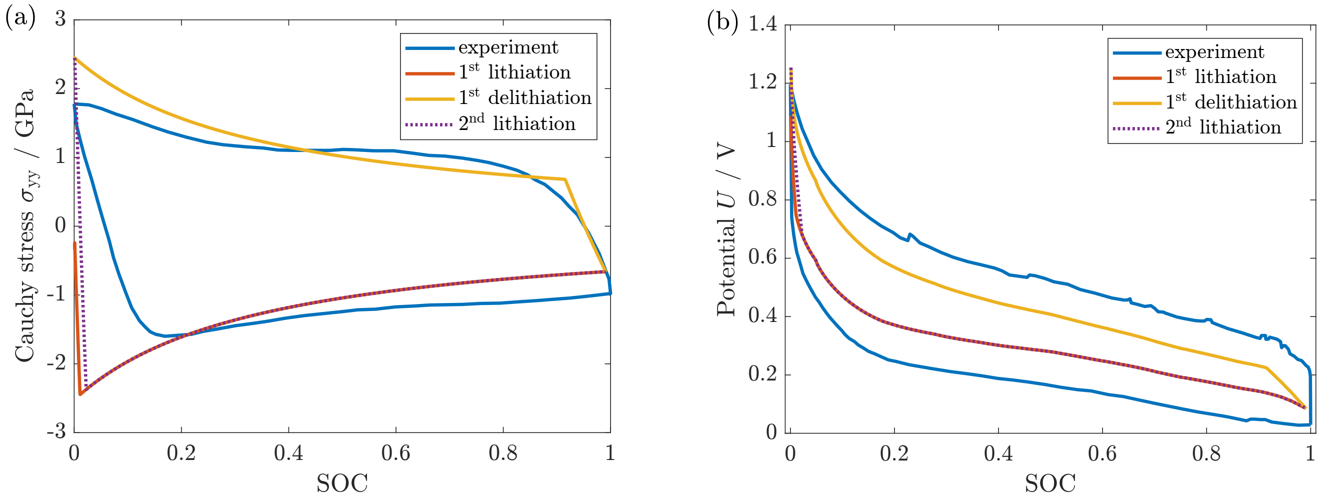


FIG. S2. Simulation of thin-film silicon anode in comparison to experiment [3]. The parameters are taken from this reference. The diffusion coefficient is $D_{\mathrm{Li}} = 1 \times 10^{-13}\,\mathrm{m^2/s}$, the film thickness is $d = 250\,\mathrm{nm}$, and the current is C/4. The remaining parameters are taken from Table S1. (a) Stress hysteresis generated by restricted expansion. The simulation can reasonably reproduce the experimental data. (b) Stress hysteresis due to large stresses. The simulation underestimates the size of the hysteresis but reproduces its shape.

## SIII. ELASTOPLASTIC SILICON PARTICLE WITH CONSTRAINTS

As seen for silicon thin films, a restricted expansion leads to large stresses. Thus, we investigate the stress of a simplified silicon nanoparticle, which is restricted by a rigid border in two directions. With this setup, we model the situation of silicon nanoparticles inside an electrode, where other electrode particles restrict the expansion. When the particle gets in contact with the wall during lithiation, large stresses arise and plastic flow starts to occur almost immediately. As illustrated in Fig. S3, this irreversibly deforms the particle, squeezing in the direction where free expansion is possible. After a short delithiation period, the plastically deformed particle detaches from the wall and stresses vanish due to the free expansion. Therefore, a significant stress and voltage hysteresis is visible for the first cycle in Fig. S4. However, for the subsequent lithiation and delithiation cycles, no plastic flow will occur, and the particle shows no stress or voltage hysteresis.

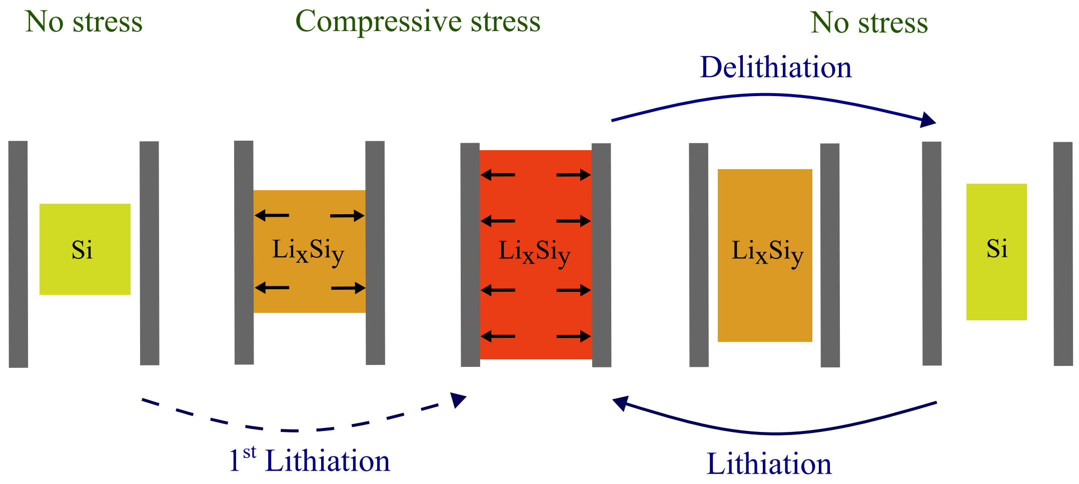


FIG. S3. Scheme of the stress inside a constrained silicon anode during first lithiation and subsequent lithiation and delithiation.

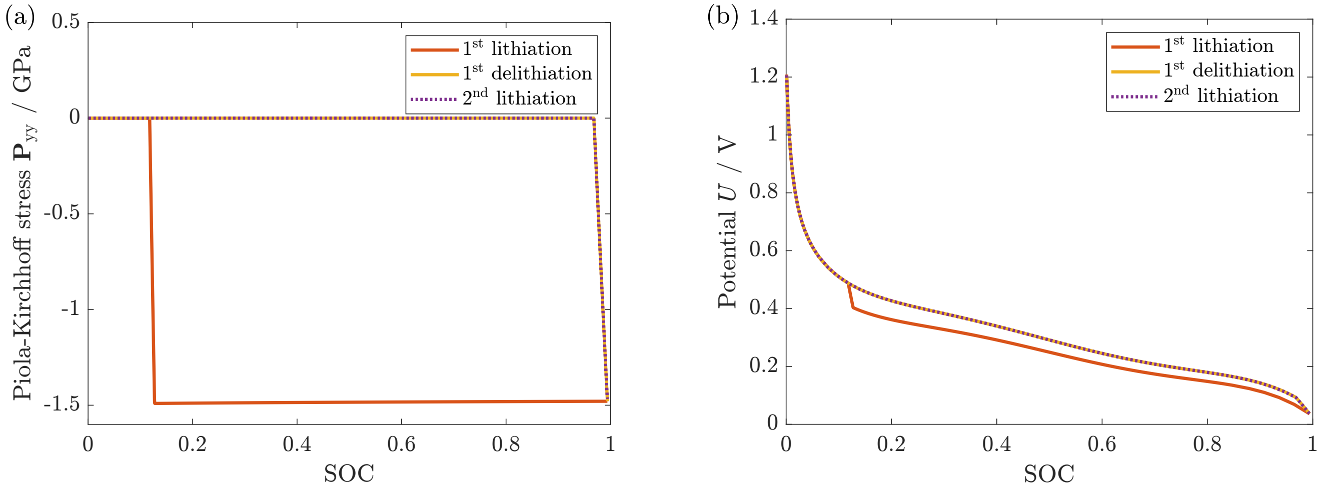


FIG. S4. Simulation of simplified nanoparticle with constraints at low C-rate. The size of the nanoparticle is 100 nm, and the distance between the fixed walls is 110 nm. (a) Stress generated by the restricted expansion. The stress vanishes when the particle is not in contact with the constraints. (b) Potential simulated for the constrained nanoparticle. A voltage hysteresis occurs only for the first cycle.

## SIV. ELASTOPLASTIC SILICON PARTICLE WITHOUT CONSTRAINTS OR SEI

In silicon nanoparticles without SEI and any borders, stress can only arise due to concentration gradients generated by the slow diffusion of lithium inside the silicon particle. To prevent underestimating the concentration gradients, we choose a small value of the diffusion coefficient of lithium in silicon reported in the literature, $D_{\mathrm{Li}} = 10^{-17}\,\mathrm{m^2 s^{-1}}$ [10]. We simulate slow lithiation and delithiation with C/20 of a silicon nanoparticle with radius $r = 50\,\mathrm{nm}$. The results shown in black in Fig. S5 reveal only a minor hysteresis in the stress and a vanishing voltage hysteresis. Therefore, slow diffusion can not explain the voltage hysteresis observed for silicon nanoparticles at C-rates as low as C/20.

To enhance the effect of concentration gradients, we increase the current to 1C. Figure S5 depicts the results for fast cycling as colored lines. Only for this high current do we find a significant stress and voltage hysteresis.

We illustrate the outcome of the simulation in Fig. S5 in comparison to the open-circuit voltage hysteresis observed via GITT measurement. Our simulation does not show a stress or voltage hysteresis after relaxation. However, we depict the experimental open-circuit voltage hysteresis in order to estimate the size of the simulated voltage hysteresis. We find that even for fast cycling with 1C the observed hysteresis is smaller than the experimental voltage hysteresis observed after relaxation.

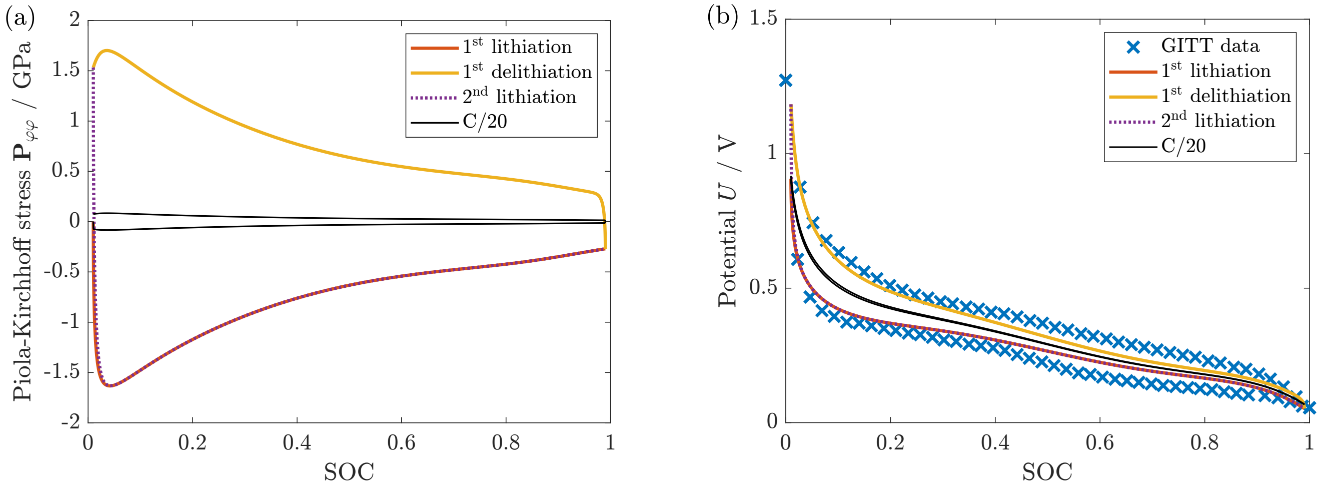


FIG. S5. Simulation of a freely expanding elastoplastic silicon nanoparticle for fast cycling with 1C (colored lines) in comparison to slow cycling with C/20 (black lines). (a) Stress hysteresis generated by concentration gradients. (b) Simulated voltage hysteresis compared to experimental GITT data [11].

## SV. PLETT MODEL

The Plett model [12–14] considers the measured potential as the sum of the mean open-circuit voltage $U_0(\mathrm{SOC})$, half of the width of the voltage hysteresis measured between lithiation and delithiation $H(\mathrm{SOC})$, and the hysteresis state $h(\mathrm{SOC})$ defined between -1 and 1 as

$$U = U_0(\mathrm{SOC}) + H(\mathrm{SOC}) \cdot h(\mathrm{SOC}). \tag{S13}$$

The Plett model defines the transition between the potential curves observed for lithiation and delithiation. It is a phenomenological model described by the differential equation

$$\frac{dh(\mathrm{SOC})}{d\mathrm{SOC}} = -k(\mathrm{SOC}) \left(1 + \mathrm{sgn}\left(\frac{d\mathrm{SOC}}{dt}\right) h(\mathrm{SOC})\right). \tag{S14}$$

The velocity of the transition between the two hysteresis paths is determined by the parameter $k$, which depends on the SOC. As a simple relation, we set $k(\mathrm{SOC}) = 40/(1 + 4 \cdot \mathrm{SOC})$.

## SVI. SEI WITH NEWTONIAN VISCOSITY

For the description of the viscosity of the SEI in our study, we apply a power-law shear-thinning behavior. Here, we evaluate the influence of Newtonian behavior, where the viscosity does not depend on the strain rate. Figure S6(a) reveals, that the size of the viscous contribution to the hysteresis decreases in our simulation with increasing SOC. The decline is produced by a decreasing strain rate, as the volume increases linearly with SOC. In comparison, the shear-thinning reduces this change in the hysteresis size and agrees better with the experimental data. According to Fig. S6(b), the Newtonian behavior possesses a similar timescale compared to the shear-thinning model used in our studies.

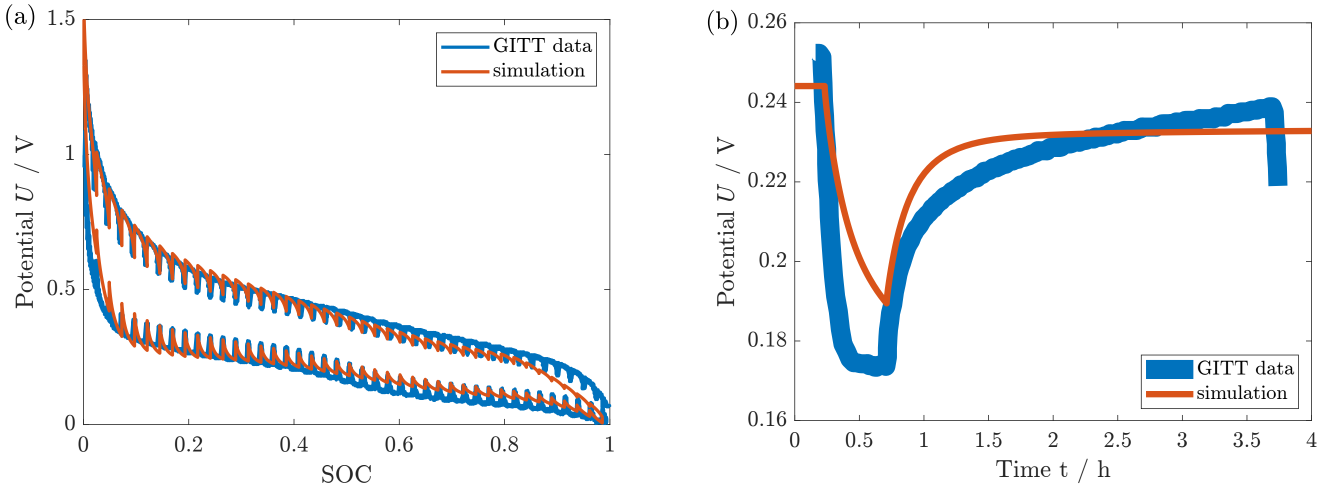


FIG. S6. Impact of Newtonian visco-elastoplastic SEI with viscosity $\eta_{\mathrm{SEI}} = 1.25 \times 10^{14}$ Pa s on the silicon potential. (a) Voltage hysteresis generated by a Newtonian visco-elastoplastic SEI for small currents and after relaxation in comparison to GITT measurement [11]. (b) Simulation of lithiation pulse and rest time in comparison to a single GITT pulse [15].

## SVII. ADDITIONAL FIGURES FOR PARAMETER STUDY

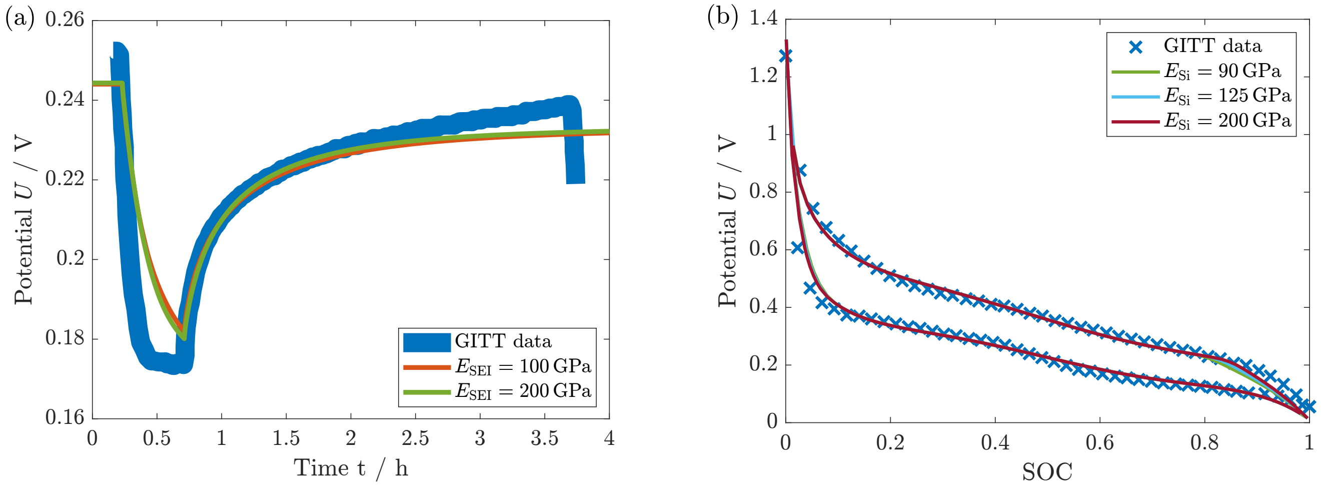


FIG. S7. Variation of Young's modulus of the SEI and the silicon particle due to nanoscale effects. (a) Variation of $E_{SEI}$ for constant $E_{Si}$. Simulation of a single GITT pulse in comparison to experimental data [15]. As the lowest value $E_{SEI} = 10$ GPa does not reproduce the voltage hysteresis, we cannot include this parameter in the figure. (b) Variation of $E_{Si}$ for constant $E_{SEI}$. Simulation of the voltage hysteresis in comparison to experimental data [11].

## SVIII. PARAMETERS

| **Parameter** | **Value** | **Reference** |
|---|---|---|
| **Silicon** | | |
| Nanoparticle radius $R$ | 50 nm | estimated [11] |
| Solid state diffusion coefficient in silicon $D_{Li}$ | $1 \times 10^{-17}$ $m^2/s$ | [10] |
| Young's modulus $E_{Si}$ | 200 GPa | estimated [16, 17] |
| Poisson's ratio $\nu_{Si}$ | 0.22 | [18] |
| Yield stress $\sigma_{Y,Si}$ | 3 GPa | fit |
| Maximum lithium concentration in Si $c_{Li,max}$ | $311 \times 10^3$ $mol/m^3$ | [19] |
| Lithium molar volume in Si $v_{Li}$ | $9 \times 10^{-6}$ $m^3/mol$ | [20] |
| Charging rate | 1/20 C | [11] |
| **SEI** | | |
| SEI thickness $L_{SEI}$ | 20 nm | estimated [21] |
| Young's modulus $E_{SEI}$ | 100 GPa | estimated [22, 23] |
| Poisson's ratio $\nu_{SEI}$ | 0.3 | [22] |
| Yield stress $\sigma_{Y,SEI}$ | 2.5 GPa | fit |
| Newtonian viscosity $\eta_{SEI}$ | $125 \times 10^{12}$ Pa s | fit |
| Shear-thinning viscosity $\eta_{SEI,0}$ | $15 \times 10^9$ Pa $s^n$ | fit |
| Shear-thinning exponent $n$ | 0.15 | estimated [24] |
| **Universal constants and other parameters** | | |
| Temperature $T$ | 298 K | |
| Faraday constant $F$ | 96 485 C/mol | |
| Universal gas constant $R_{gas}$ | 8.314 J/(mol K) | |

TABLE S1. List of the simulation parameters.

[1] L. Kolzenberg, A. Latz, and B. Horstmann, Chemo-Mechanical Model of SEI Growth on Silicon Electrode Particles, Batteries & Supercaps **5**, 1 (2022).

[2] L. Baggetto, J. Oudenhoven, T. van Dongen, J. Klootwijk, M. Mulder, R. Niessen, M. de Croon, and P. Notten, On the electrochemistry of an anode stack for all-solid-state 3D-integrated batteries, Journal of Power Sources **189**, 402 (2009).

[3] V. A. Sethuraman, M. J. Chon, M. Shimshak, V. Srinivasan, and P. R. Guduru, In situ measurements of stress evolution in silicon thin films during electrochemical lithiation and delithiation, Journal of Power Sources **195**, 5062 (2010).

[4] V. A. Sethuraman, V. Srinivasan, A. F. Bower, and P. R. Guduru, In Situ Measurements of Stress-Potential Coupling in Lithiated Silicon, Journal of The Electrochemical Society **157**, A1253 (2010).

[5] V. A. Sethuraman, V. Srinivasan, and J. Newman, Analysis of Electrochemical Lithiation and Delithiation Kinetics in Silicon, Journal of The Electrochemical Society **160**, A394 (2013).

[6] M. W. Verbrugge, D. R. Baker, X. Xiao, Q. Zhang, and Y.-T. Cheng, Experimental and Theoretical Characterization of Electrode Materials that Undergo Large Volume Changes and Application to the Lithium–Silicon System, The Journal of Physical Chemistry C **119**, 5341 (2015).

[7] I. Yoon, D. P. Abraham, B. L. Lucht, A. F. Bower, and P. R. Guduru, In Situ Measurement of Solid Electrolyte Interphase Evolution on Silicon Anodes Using Atomic Force Microscopy, Advanced Energy Materials **6**, 1600099 (2016).

[8] B. Lu, Y. Song, Q. Zhang, J. Pan, Y.-T. Cheng, and J. Zhang, Voltage hysteresis of lithium ion batteries caused by mechanical stress, Physical Chemistry Chemical Physics **18**, 4721 (2016).

[9] D. R. Baker, M. W. Verbrugge, and X. Xiao, An approach to characterize and clarify hysteresis phenomena of lithium-silicon electrodes, Journal of Applied Physics **122**, 165102 (2017).

[10] J. Li, X. Xiao, F. Yang, M. W. Verbrugge, and Y.-T. Cheng, Potentiostatic Intermittent Titration Technique for Electrodes Governed by Diffusion and Interfacial Reaction, The Journal of Physical Chemistry C **116**, 1472 (2012).

[11] K. Pan, F. Zou, M. Canova, Y. Zhu, and J.-H. Kim, Systematic electrochemical characterizations of Si and SiO anodes for high-capacity Li-Ion batteries, Journal of Power Sources **413**, 20 (2019).

[12] G. L. Plett, Extended Kalman filtering for battery management systems of LiPB-based HEV battery packs, Journal of Power Sources **134**, 262 (2004).

[13] C. P. Graells, M. S. Trimboli, and G. L. Plett, Differential hysteresis models for a silicon-anode Li-ion battery cell, in *2020 IEEE Transportation Electrification Conference & Expo (ITEC)*, Vol. 1 (IEEE, 2020) pp. 175–180.

[14] D. Wycisk, M. Oldenburger, M. G. Stoye, T. Mrkonjic, and A. Latz, Modified Plett-model for modeling voltage hysteresis in lithium-ion cells, Journal of Energy Storage **52**, 105016 (2022).

[15] K. Pan, *Dissertation*, Ph.D. thesis, Ohio State University (2020).

[16] M. Nasr Esfahani and B. E. Alaca, A Review on Size-Dependent Mechanical Properties of Nanowires, Advanced Engineering Materials **21**, 1900192 (2019).

[17] D.-M. Tang, C.-L. Ren, M.-S. Wang, X. Wei, N. Kawamoto, C. Liu, Y. Bando, M. Mitome, N. Fukata, and D. Golberg, Mechanical Properties of Si Nanowires as Revealed by in Situ Transmission Electron Microscopy and Molecular Dynamics Simulations, Nano Letters **12**, 1898 (2012).

[18] V. Shenoy, P. Johari, and Y. Qi, Elastic softening of amorphous and crystalline Li–Si Phases with increasing Li concentration: A first-principles study, Journal of Power Sources **195**, 6825 (2010).

[19] A. Verma, A. A. Franco, and P. P. Mukherjee, Mechanistic Elucidation of Si Particle Morphology on Electrode Performance, Journal of The Electrochemical Society **166**, A3852 (2019).

[20] R. Koerver, W. Zhang, L. de Biasi, S. Schweidler, A. O. Kondrakov, S. Kolling, T. Brezesinski, P. Hartmann, W. G. Zeier, and J. Janek, Chemo-mechanical expansion of lithium electrode materials – on the route to mechanically optimized all-solid-state batteries, Energy & Environmental Science **11**, 2142 (2018).

[21] J. Zheng, H. Zheng, R. Wang, L. Ben, W. Lu, L. Chen, L. Chen, and H. Li, 3D visualization of inhomogeneous multi-layered structure and Young's modulus of the solid electrolyte interphase (SEI) on silicon anodes for lithium ion batteries, Phys. Chem. Chem. Phys. **16**, 13229 (2014).

[22] H. Shin, J. Park, S. Han, A. M. Sastry, and W. Lu, Component-/structure-dependent elasticity of solid electrolyte interphase layer in Li-ion batteries: Experimental and computational studies, Journal of Power Sources **277**, 169 (2015).

[23] Y. Chai, W. Jia, Z. Hu, S. Jin, H. Jin, H. Ju, X. Yan, H. Ji, and L.-J. Wan, Monitoring the mechanical properties of the solid electrolyte interphase (SEI) using electrochemical quartz crystal microbalance with dissipation, Chinese Chemical Letters **32**, 1139 (2021).

[24] W. S. LePage, Y. Chen, E. Kazyak, K.-H. Chen, A. J. Sanchez, A. Poli, E. M. Arruda, M. D. Thouless, and N. P. Dasgupta, Lithium Mechanics: Roles of Strain Rate and Temperature and Implications for Lithium Metal Batteries, Journal of The Electrochemical Society **166**, A89 (2019).
